# Supplementary material for: Modeling the origin of urban output scaling laws
Source: arXiv:1712.00476 source file (2019-08-26)
Supplement: Supplementary file 1 [file Yang_SM.pdf]

# Supplemental Material for
# "Modeling the origin of urban output scaling laws"

V. Chuqiao Yang, Andrew V. Papachristos, and Daniel M. Abrams

## Contents


**1 Data Sources** **1**

**2 Differences among scaling relationships** **3**

**3 Parameter fitting and discussions** **3**

**4 Calculation of best-fitting power law exponent** **8**

**5 Model's fits to all seven types of crimes** **8**

**6 Comparison with power-law models** **8**

**7 Secondary correction** **10**

**8 Additional mathematical derivations** **10**

**9 Model's application to patent scaling** **13**

**10 Code and data availability** **14**


## 1 Data Sources

### US crime statistics by MSA

US crime statistics by MSA are obtained from Table 6 of the Federal Bureau of Investigation (FBI) publication *Crime in the United States* for years 1999–2012. The data can be accessed online at `https://ucr.fbi.gov/ucr-publications` (as of January 17, 2017). For each year, population, as well as crime rates for seven types of crimes (murder, forcible rape, robbery, aggravated assault, burglary, larceny-theft, and motor vehicle theft) are reported for between 260 and 360 MSA's. We used a total of 98 data sets (14 years $\times$ 7 crime types).

## Co-offending data from the Chicago Police Department

We estimate the group size of crime by compiling a new data set of arrest records for 352,705 crime incidents from the city of Chicago, IL from 1999 to 2012. The data were provided to one of the authors through a memorandum of understanding with the Chicago Police Department. Data are recorded at the incident level and include detailed information on each arrest, including the charge (e.g., motor vehicle theft, assault, robbery, etc.) as well as individual information on the offender(s). Co-offending is defined as two or more individuals being charged for the same offence as co-perpetrators, such as when two individuals steal a car together, sell drugs together, or rob someone together. We define "group size" as the number of offenders participating in a single crime, and without regard to any indication of a formal criminal group, such as a street gang. For example, if three people were involved in a motor vehicle theft, the group would have a size of three. Data used in the present analyses are derived from a cross-tabulation of offence type by group size for all offences from 1999 to 2012. Some summary of the dataset can be found in Table S1. A plot of mean group sizes by year and bootstrapped estimation of the 95% confidence intervals is shown in Figure S1.

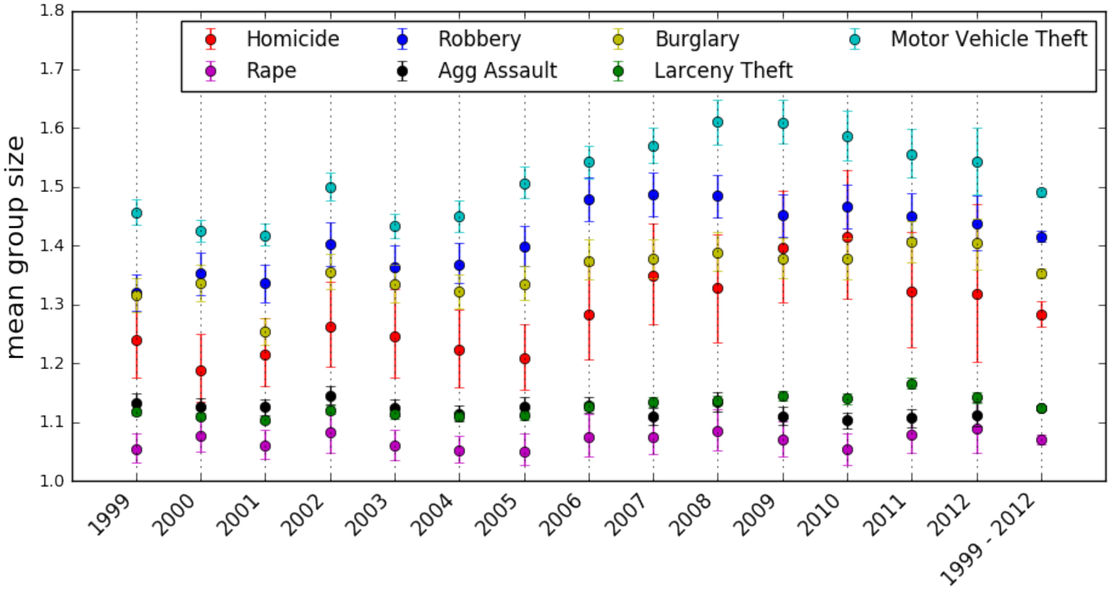


**Figure S1:** Mean group sizes (with 95% confidence interval as vertical error bars) for seven types of crimes over time extracted from the Chicago Police Department arrest records.

## Co-offending group size from the National Incident-Based Reporting System

A dataset we use to extract co-offending group size is the Uniform Crime Reporting Program Data: National Incident-Based Reporting System (NIBRS) 2014 through the National Archive of Criminal Justice (`https://www.icpsr.umich.edu/icpsrweb/NACJD/studies/36398`), accessed in March 2017 [1]. We join the "offense" and "offender" tables of the data on incident number and state code. Based on descriptions in the codebook, we identify crime

types of each instance by the UCR offence code using the following matching—murder: 09A, robbery: 120, rape: 11A, aggravated assault: 13A, burglary: 220, larceny-theft: 23A - 23H, and motor-vehicle theft: 240.

The co-offending group size for an offence is defined by the number of unique offenders reported in this offence. A total of 968,962 instances were available from this dataset for the categories of crimes of interest. A comparison of the values extracted from the NIBRS dataset with the Chicago dataset is shown in Table S1. Please note that the methodology of this dataset is different from that of the Chicago one: the Chicago dataset reports only arrested offenders, while the NIBRS includes voluntary instance reports from police departments, regardless of whether the offenders were arrested. Thus the values of co-offending group size are expected to have small systematic differences between these two datasets. Additionally, it is important to note that the Chicago Police Department does not participate in NIBRS, so the two datasets are mutually exclusive.

| | Chicago PD arrest record | NIBRS |
|---|---|---|
| Homicide | 1.28 | 1.58 |
| Rape | 1.07 | 1.29 |
| Robbery | 1.41 | 1.74 |
| Agg. assault | 1.12 | 1.33 |
| Burglary | 1.35 | 1.41 |
| Larceny-theft | 1.12 | 1.29 |
| Motor vehicle theft | 1.49 | 1.36 |
| Year | 1999 - 2012 | 2014 |
| Number of instances | 352,705 | 968,962 |

**Table S1:** Average co-offending group size for various types of crime in the Chicago PD arrest record and the NIBRS dataset.

### The Enron corpus

We used email communication records from a corpus derived from Enron Corporation to check the plausibility of the parameter $\alpha$ in our rank-frequency distribution, $\rho$. The Enron corpus contains 517,431 emails sent by 151 employees of the Enron Corporation. This dataset was downloaded from `http://www.cs.cmu.edu/~enron/` in November 2014 [2].

## 2 Differences among scaling relationships

Table S2 summarizes the differences in some examples of urban outputs, including crimes broken down by category.

## 3 Parameter fitting and discussions

Our model has three parameters that must be fit from data: $s$, $\alpha$, and a multiplicative prefactor. The first two parameters are assumed universal across all data sets, and the third

| Urban output | Exponent | 95% CI | Year |
|---|---|---|---|
| Larceny theft [3] | 0.98 | [0.95, 1.02] | 2002 |
| Rape [3] | 0.98 | [0.92, 1.04] | 2002 |
| Burglary [3] | 1.01 | [0.96 , 1.05] | 2002 |
| Total wages [4] | 1.12 | [1.09, 1.13] | 2002 |
| Aggravated assault [3] | 1.13 | [1.06 , 1.20] | 2002 |
| Murder [3] | 1.22 | [1.14, 1.30] | 2002 |
| New AIDS cases [4] | 1.23 | [1.18, 1.29] | 2002–2003 |
| New patents [4] | 1.27 | [1.25, 1.29] | 2001 |
| Motor vehicle theft [3] | 1.32 | [1.27 , 1.38] | 2002 |
| Robbery [3] | 1.38 | [1.31 , 1.45] | 2002 |

**Table S2:** Best fitting power law exponent for scaling relations for various urban outputs. The differences among them can be pronounced.

is unique for each. For $N$ sets of data, we thus require $N + 2$ parameters to be fitted. We find the values of the two global parameters ($s$ and $\alpha$) by minimizing the sum of the 2-norm error across all 98 datasets. The model parameter $n$ is set by the average number of partners calculated from the average co-offending group sizes in data. Fig. S2 shows the landscape of 2-norm error in the neighbourhood of the optimal parameter pair (using NIBRS as the group size input). Interestingly, we observe a "valley" in the error landscape, showing that there may be an effective parameter that is a nonlinear combination of $\alpha$ and $s$. One potential explanation is that one can meet more distinct individuals by simply sampling more people (increasing $s$), or by change one's social interaction pattern to interact with more "weak ties" (decreasing $\alpha$). We have also checked the robustness of the parameter fit by minimizing the 1-norm, and we found similar best fitting parameter ($s = 2.8 \times 10^6$, $\alpha = 0.93$), and we observe a similar error landscape.

## Validating fitted $\alpha$ with Enron data

To check if the fitted parameters are plausible, we compare the power law exponent $\alpha$ for contact frequency that results from our parameter fit to an empirical estimate using the Enron email corpus. Although the two interaction networks are quite different (face-to-face casual contacts versus corporate email communications), we see this as a necessary minimal "sanity check" to ensure that our parameter optimization is not beyond the bounds of credibility. From the emails in the "sent_item" folder of each user, we extract sender and receivers' email addresses, as well as the length of each email in characters, excluding white spaces and quoted text in forwarded messages and replies. Some examples of the length of communication to contact vs rank of the contact are shown in Fig. S3-left.

We excluded those senders with too few contacts ($< 100$). The communication length vs rank relation may be approximated as a power law, with the exception of the low-frequency contacts at larger ranks. We used the communication length vs. rank relation (up to rank 100) to fit the power law exponent $-\alpha$ for each sender. Some examples of the relations are shown in Fig. S3-right. The distribution of those $\alpha$ is shown in Fig. S4. The best fitting $\alpha$ from fitting the model to crime scaling data, while using the Chicago data as input group

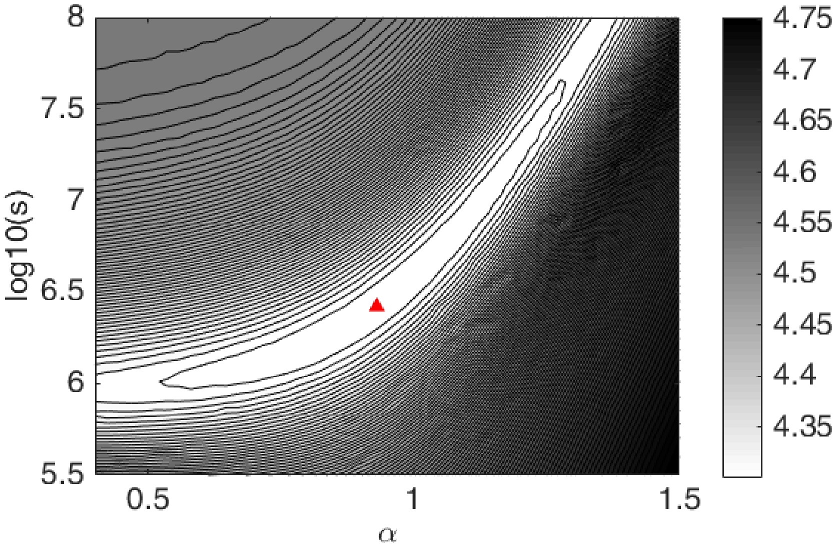


**Figure S2:** Error landscape for the global parameter optimization problem. Contours show lines of constant 2-norm for the difference between theory and data over all datasets. The red triangle shows optimized parameters giving the best fit.

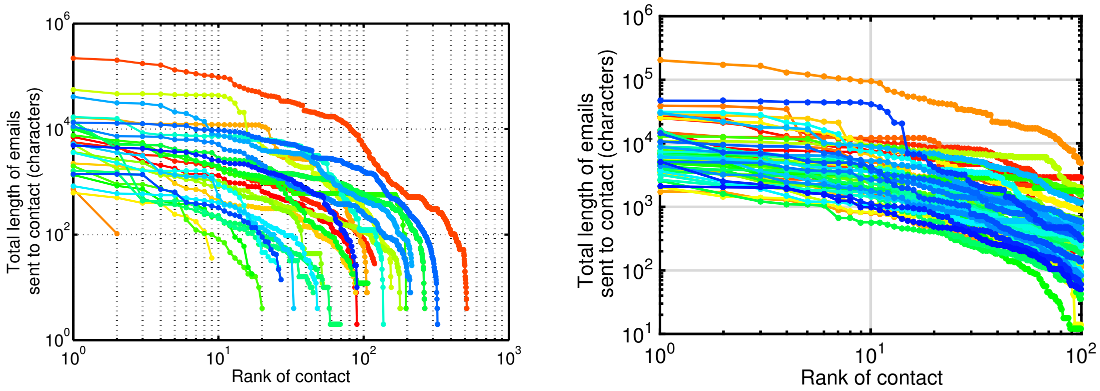


**Figure S3:** Left: Examples of the amount of contact vs. rank for 30 randomly selected individuals in Enron database. Right: The amount of contact vs. rank of contact distribution for the individuals in the dataset with more than 100 contacts. The curves for small ranks can be roughly approximated as power laws, though not perfectly.

size is 0.69. The best fitting $\alpha$ while using the NIBRS group size as input, is 0.93, both are plausibly consistent with the distribution.

## Discussion of the functional form of $\rho(x)$

When comparing our model with data, we assume $\rho(x) \sim x^{-\alpha}$. The motivation is to avoid assumptions about the structure of social networks, since that is a complex question on its own and is not central to this paper's discussion. Although some network structures can result in $\rho(x) \sim x^{-\alpha}$, it is not a necessary condition to reach our major conclusions. It

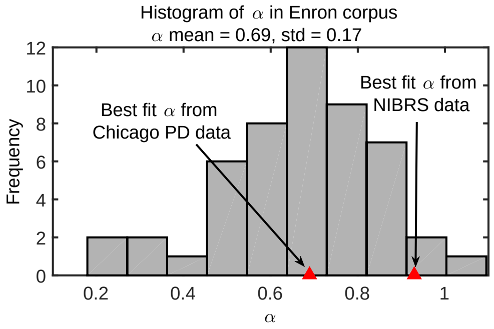


**Figure S4:** Histogram of fitted $\alpha$ for all individuals with more than 100 contacts in the Enron email database, compared with $\alpha$ found by fitting our model to crime scaling data while using two independent datasets as group size input. Both *alpha* values found are plausibly consistent with the distribution.

is important to note that relaxing this assumption to general non-increasing $\rho(x)$ (which is by definition true for a rank-probability distribution) does not affect the fundamental predictions of this work—people in larger cities meet more unique individuals, and the more participants an act requires, the greater the superlinearity. Other choices produce similar qualitative results. Figure S5 compares predictions using some alternative functional forms of $\rho$ with data. These alternative functional forms are also able to predict both the superlinear scaling (left column of Figure S5) and nearly linear scaling (right column of Figure S5).

Figure S5-A and B assume $\rho$ to be a decaying log normal function,

$$\rho(x) = \frac{1}{x\sigma\sqrt{2\pi}} \exp\left[-\frac{(\ln(x)-\mu)^2}{2\sigma^2}\right].$$

To ensure that $\rho(x)$ is a non-increasing function, we set $\rho(x)$'s maximum to be at $x = 1$, the starting point of the 1D rank space, which constrains the parameters to be $\mu = \sigma^2$. Figure S5-A and B shows scaling predictions for parameters $\mu = \sigma^2 = 10$, and $s = 2.63 \times 10^6$ (same $s$ as used in the main text).

In Figure S5-C and D, we assume $\rho$ to be a piecewise constant function representing the "circles of acquaintanceship" as proposed by Dunbar [5], with four discrete jumps in interaction probability. We use Dunbar's estimation and set the sizes of the circles to be 5, 15, 50 and 150 people. We assume the interaction frequency decreases by a factor of 10 when moving from one circle to the next:

$$\rho(x) = m(N) \times \begin{cases} 10^4 & 1 \leq x \leq 5 \\ 10^3 & 5 < x \leq 15 \\ 10^2 & 15 < x \leq 50 \\ 10^1 & 50 < x \leq 150 \\ 10^0 & 150 < x \leq N \end{cases},$$

where $m(N)$ is a multiplicative normalization factor so that $\int_1^N \rho(x)dx = 1$. Figure S6 visualizes these alternative $\rho$ functions and compares with the power-law assumption in the main text. Figure S5-C and D also uses the same $s$ parameter as in the main text.

Generalizing beyond these numerical simulations, Section 8 demonstrates that $u(N)$ must be a non-decreasing function of $N$ even without any assumption regarding the functional form for $\rho$. Thus the qualitative conclusions of the main text hold for general $\rho$.

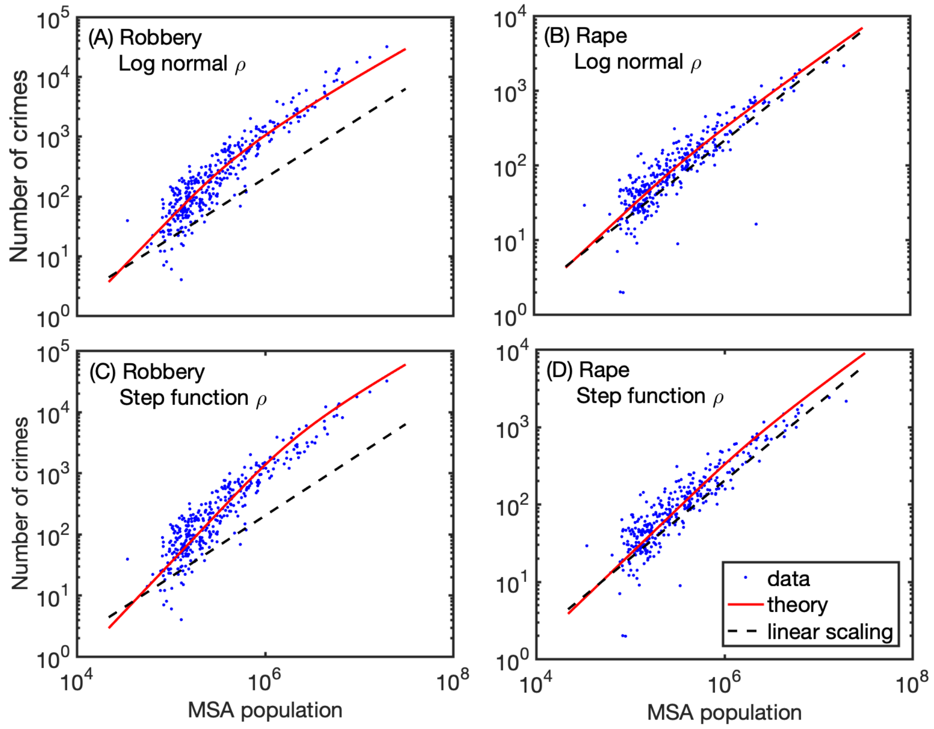


**Figure S5:** Example results for an alternative functional forms of $\rho$, where $\rho$ takes the form of (A, B) a log normal function, or (C, D) a piecewise constant function denoting circles of acquaintanceship with decaying likelihood of interaction in each circle.

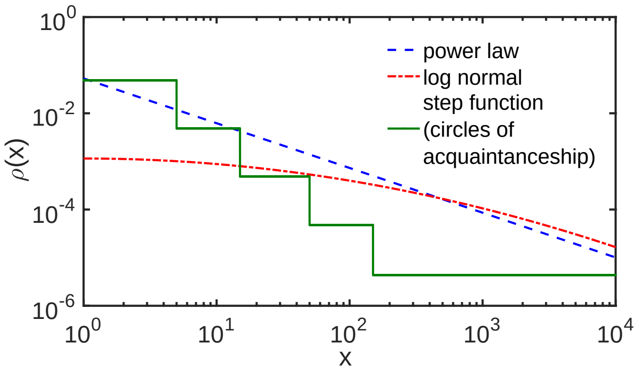


**Figure S6:** Comparing the power-law function $\rho$ with alternative functional forms that generate results as shown in Figure S5. Parameter values used here are the same as those used to generate the scaling predictions.

# 4 Calculation of best-fitting power law exponent

We quantify the degree of superlinear scaling using the best fitting power-law exponent in the scaling relationship of MSA total output vs. MSA population, consistent with Bettencourt et. al [4]. The exponent is the slope of the linear fit $\log(y) = a_1 \log(x) + a_2$, where $x$ and $y$ are the MSA population (horizontal axis) and amount of output (vertical axis) respectively. The parameters $a_1$ and $a_2$ are to be fitted from the data; $a_1$ is the fitted power law exponent, and thus $a_1 - 1$ is the superlinearity shown in Fig. 4 of the main text.

The superlinearity for the theory lines in Fig. 4 is calculated as follows. Since the theory does not predict a power law relationship, we first calculate the theory's prediction of total output for each MSA population in the data. We then fit those predictions to a power law in the same way we fit the data to arrive at the estimate of superlinearity.

The authors are aware of the criticisms for linear fit on the log scale [6], and are motivated by them to develop the non-power-law model described in the main text. The purpose of using the linear fit is not to claim a power-law relationship. Instead, we use it to arrive at an indicator to assist us comparing the steepness of the scaling relationship in the data and in the theory, and to visualize the relationship between group size and the steepness of the scaling relationship.

# 5 Model's fits to all seven types of crimes

Fig. S7 shows our theory's comparison with the 7 categories of crime in year 2012, the most recent year of data available when the research was performed, with the group size input from the NIBRS dataset. In addition, Fig. S8 shows the fit to patent data (with sources and group size input described in Sec. 9, showing year 2000, the most recent year available), suggesting that the model may be generalized to urban outputs beyond crime. Please note that for all the data displayed, the theoretical curves use the same universal set of parameters $\alpha$ and $s$. The only parameter fitted separately to each data set is a multiplicative scaling factor (see Sec. 3).

# 6 Comparison with power-law models

A recently published study [7] also hypothesizes that variation may result from the need for a number of complementary factors to come together, but assumes the scaling take on a power-law form. Our work relaxes the power-law scaling assumption, and we present empirical evidence that validates our hypotheses.

We compare our model with the power law assumption ($y = aN^b$) for each data set. The power law model uses $2N$ parameters for $N$ data sets. Our model uses $N + 2$ parameters for $N$ datasets. We use the Akaike and Bayesian Information Criteria (AIC and BIC) to measure the goodness of fit. The result is shown in Table S3. Our model has lower AIC and BIC values than the power law model, thus reaches better fit with data, accounting for the parameters used (evidence ratio based on AIC is $\exp(\frac{1}{2}\Delta\text{AIC}) \approx \exp(9000) \sim 10^{3900}$ [8], strongly supporting our simpler model).

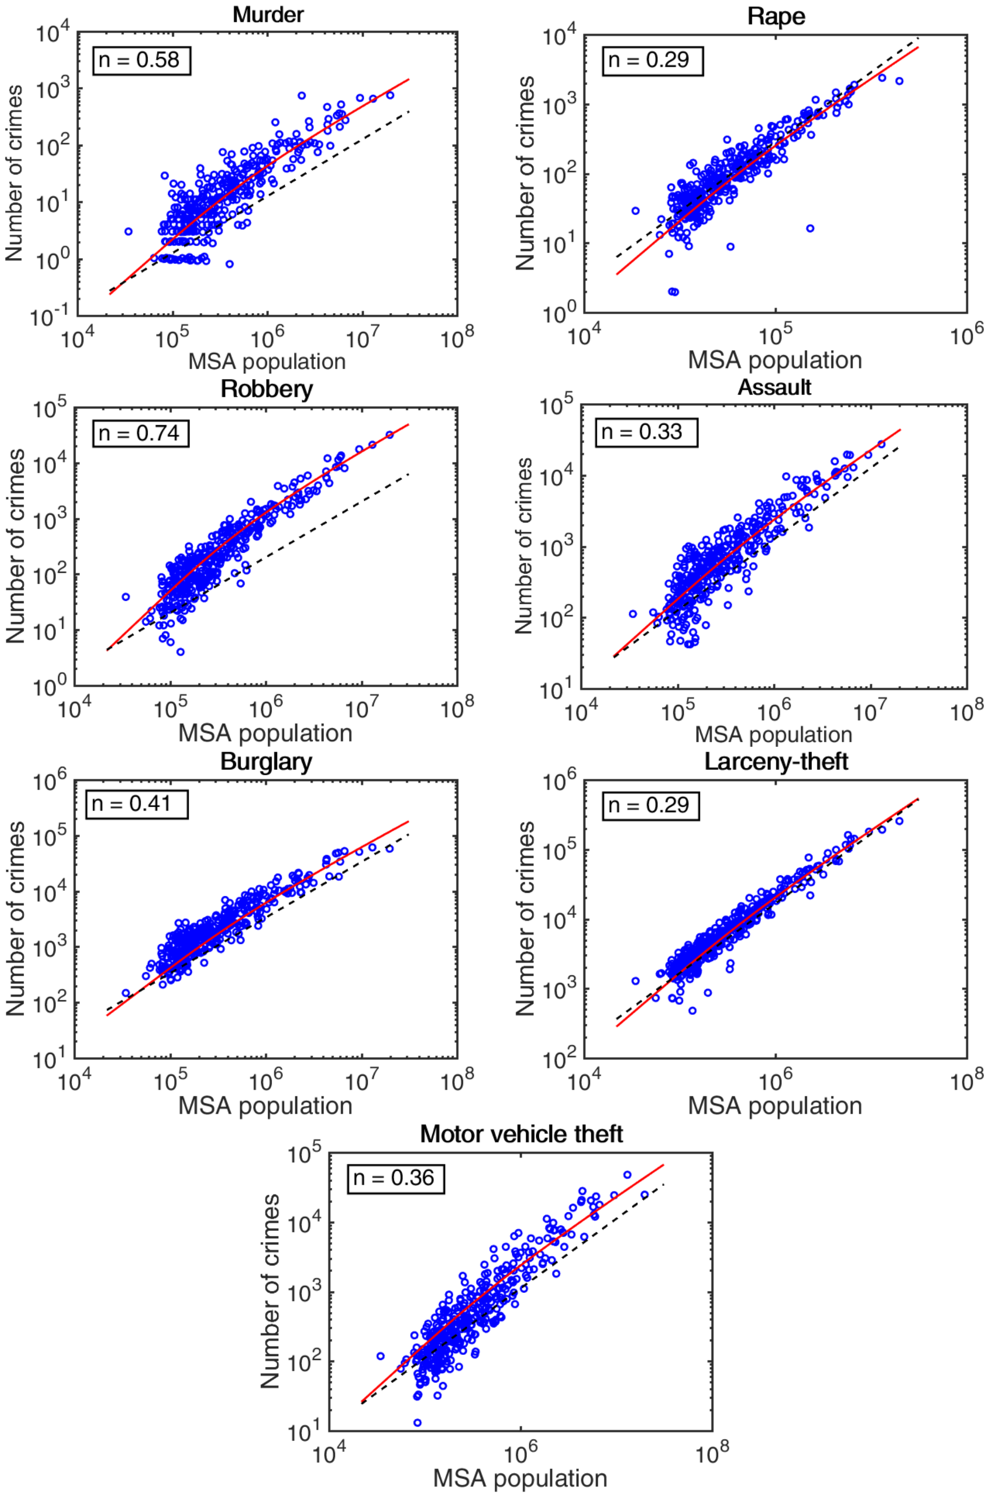


**Figure S7:** The fits of the model to all seven types of crimes and to patent data. Fits for other years are similar. In all panels, the blue dots are data points, red curves are model predictions, and the black dashed lines show linear scaling. The average number of partners $n$ is indicated on each panel.

| | AIC | BIC |
|---|---|---|
| power law model | 5.34e+05 | 5.36e+05 |
| our model | 5.16e+05 | 5.17e+05 |

**Table S3:** AIC and BIC of the two types of models with best fitting parameters

# 7 Secondary correction

Previous studies support the idea that higher wages can lead to a lower crime rate [9, 10, 11]. One theory regarding crime incentives suggests that if the gain from committing a crime exceeds the wage one would otherwise earn with the same time and effort, one would be inclined to commit a crime. Historical data support that at least some young men's behaviour is responsive to this type of crime incentive [10]. Motivated by these findings, we include a secondary correction in our prediction:

$$y(N) \propto N \cdot u^n(N) f(w(N))$$

where $w(N)$ is the average wage one would earn in a city of population $N$. Empirical data suggest that $w(N) \sim N^{0.12}$ [12]. The propensity to commit a crime decreases with increasing mean wage, so as a simple approximation we take $f$ to be the function $f(w) = 1/w$. Then

$$\begin{aligned} y(N) &\sim N \cdot u^n(N) N^{-0.12} \\ &\sim N^{0.88} \left( N - \int_1^N e^{-\rho(x;N)s} dx \right)^n . \end{aligned} \quad (1)$$

We use this model equation for comparison with the crime data sets.

# 8 Additional mathematical derivations

## Integral Approximation

Here, we find an asymptotic approximation of the integral in the expression of $u(N)$ of the main text to simplify computation of the model. We use this asymptotic approximation when validating the model with empirical data.

In main text Eq. (3), we have

$$u(N) = N - \int_1^N e^{-\rho(x)s} dx . \quad (2)$$

We would like to approximate the integral

$$I_1(N) = \int_1^N e^{-\rho(x)s} dx = \int_1^N e^{-mx^{-\alpha}s} dx ,$$

where $m = m(N)$ is a normalization constant with $m = (\alpha - 1)/(1 - N^{1-\alpha})$ if $\alpha \neq 1$; $m = 1/\ln(N)$ if $\alpha = 1$.

First, we make a change of variable, $t = x^{-\alpha}s$. Then we have

$$I_1(N) = \frac{1}{\alpha}s^{1/\alpha}\int_{N^{-\alpha}s}^{s} e^{-mt}t^{-\frac{\alpha+1}{\alpha}}dt \ . \tag{3}$$

Now we focus on the integral in (3),

$$I_2(N) = \int_{N^{-\alpha}s}^{s} e^{-mt}t^{-\frac{\alpha+1}{\alpha}}dt \ . \tag{4}$$

Then we have the relation $I_1 = s^{1/\alpha}I_2/\alpha$. Substitute $k = (\alpha+1)/\alpha$, $(k > 1)$ in (4), we have

$$I_2(N) = \int_{N^{-1/(k-1)}s}^{s} e^{-mt}t^{-k}dt \ . \tag{5}$$

Substitute $\epsilon = mN^{-1/(k-1)}s$ and $\tau = mt$, into (5), we have

$$I_2(\epsilon) = m^{k-1}\int_{\epsilon}^{ms} e^{-\tau}\tau^{-k}d\tau \ .$$

Note that the integrand $e^{-\tau}\tau^{-k}$ diverges at $\tau \to 0$ for all $k > 0$, and more importantly, it diverges with a heavy head for all $k > 1$. So the neighborhood of $\epsilon$ dominates the integral, and we can replace the upper bound by infinity with error that's only exponentially small:

$$I_2(\epsilon) \approx m^{k-1}\int_{\epsilon}^{\infty} e^{-\tau}\tau^{-k}d\tau \ . \tag{6}$$

The integral in (6) is the upper incomplete gamma function:

$$I_2(\epsilon) = m^{k-1}\Gamma(1-k,\epsilon) \ .$$

The upper incomplete gamma function, $\Gamma(a,z)$ is defined as,

$$\begin{aligned}
\text{if } a > 0: &\qquad \Gamma(a,z) = \int_{z}^{\infty} e^{-t}t^{a-1}dt \ , \\
\text{if } a < 0: &\qquad \Gamma(a,z) = \Gamma(a+1,z) - \frac{z^a}{a}e^{-x} \ .
\end{aligned}$$

The $a < 0$ recurrence relation is found using integration by parts.

Undoing the variable transformations, we have

$$I_1(N) = \frac{(s\ m)^{1/\alpha}}{\alpha}\Gamma(-\frac{1}{\alpha}, m\ N^{-\alpha}s) \ ,$$

so

$$u(N) = N - \frac{(s\ m)^{1/\alpha}}{\alpha}\Gamma(-\frac{1}{\alpha}, m\ N^{-\alpha}s) \ . \tag{7}$$

## Show $du/dN \geq 0$

Here we show that $du/dN \geq 0$ is implied even without the assumption of power law $\rho$. Let $\rho$ take on any separable form, $\rho(x;N) = m(N)f(x)$, where $f(x) \geq 0$ represents a communication pattern that is universal across cities, and $m(N)$ is a normalization factor. This assumption considers the case where individuals of identical social interaction pattern reside in cities of different sizes.

Note that the population in the 1-D space is ordered by decreasing probability of interaction. Thus, by definition, $f'(x) \leq 0$.

From the main text Eq. (6), we have

$$u(N) = N - \int_1^N e^{-\rho(x;N)s} dx \ . \tag{8}$$

Since the integral is dominated by small $\rho s$ values, we approximate (8) with a Taylor expansion near $\rho s = 0$:

$$\begin{aligned} u(N) &\approx N - \int_1^N \left(1 - \rho(x;N)s + \frac{1}{2}(\rho(x;N)s)^2\right) dx \\ &= 1 + s\int_1^N \rho(x;N)dx - \frac{s^2}{2}\int_1^N \rho^2(x;N)dx \\ &= 1 + s - \frac{s^2}{2}\int_1^N \rho^2(x;N)dx \ . \end{aligned} \tag{9}$$

Then

$$\frac{du}{dN} = -\frac{s^2}{2}\frac{d}{dN}\int_1^N \rho^2(x;N)dx \ . \tag{10}$$

Using Leibniz's rule for differentiation under the integral sign, we have

$$\frac{du}{dN} = -\frac{s^2}{2}\left[\int_1^N \frac{d}{dN}\rho^2(x;N)dx + \rho^2(N,N)\right] \ . \tag{11}$$

Let $\rho = m(N)f(x)$, denote $Q = \int_1^N \frac{d}{dN}\rho^2(x;N)dx + \rho^2(N,N)$. Then

$$\frac{d}{dN}\rho^2(x;N) = 2f^2(x)m(N)\frac{dm(N)}{dN} \ ,$$

and

$$Q = 2m\frac{dm}{dN}\int_1^N f^2(x)dx + f^2(N)m^2(N) \ . \tag{12}$$

Since the normalization factor $m$ satisfies

$$m(N) = \frac{1}{\int_1^N f(x)dx} \ ,$$

then

$$\frac{dm}{dN} = -\frac{f(N)}{(\int_1^N f(x)dx)^2}.$$

Substituting into (12), we have

$$
\begin{aligned}
Q &= -2\frac{f(N)}{(\int_1^N f(x)dx)^3}\int_1^N f(x)^2 dx + \frac{f^2(N)}{(\int_1^N f(x)dx)^2} \\
&= \frac{f(N)\left[f(N)\int_1^N f(x)dx - 2\int_1^N f^2(x)dx\right]}{(\int_1^N f(x)dx)^3} .
\end{aligned}
$$

Define $S(N) = f(N)\int_1^N f(x)dx - 2\int_1^N f^2(x)dx$ (the bracketed expression above). Since $f(x) \geq 0$ and $\rho$ normalizable, the denominator of $Q$ must be positive. In order to show $du/dN = -s^2 Q/2 \geq 0$, we need to show $S \leq 0$. It's clear that $S(1) = 0$. Now it suffices to show $dS/dN \leq 0$:

$$
\begin{aligned}
\frac{dS}{dN} &= f'(N)\int_1^N f(x)dx + f^2(N) - 2f^2(N) \\
&= f'(N)\int_1^N f(x)dx - f^2(N) . \qquad (13)
\end{aligned}
$$

By definition, $f(x)$ is a non-increasing function, i.e., $f'(N) \leq 0$. Examining (13) with this in mind, we observe that

$$\frac{dS}{dN} \leq 0.$$

So $S(N) \leq 0$ for all $N > 1$ and therefore $Q \leq 0$ for all $N > 1$. Thus

$$\frac{du}{dN} = -\frac{s^2}{2}Q \geq 0 .$$

# 9 Model's application to patent scaling

In the main text, we discussed possible extensions of our model to urban outputs beyond crime. In this section, we show results comparing our model (with parameters found by fitting to the crime data) to the scaling of patents, and find good agreement.

We first compute the average group size for patents from the National Bureau of Economic Research (NBER) database [13]. The data were downloaded from http://www.nber.org/patents in July 2016. The data comprise detailed information on almost 3 million U.S. patents granted between January 1963 and December 1999. Here the group size is defined as the number of authors on a patent. Note that this dataset does not aggregate patent information by MSA. We also extract the patent scaling data (number of patents by MSA) from Bettencourt et al. [14] Fig. 1 using the GetData Graph Digitizer software.

We use the average group size found in the NBER database as the input of group size $(n+1)$ in our model. We also use the best fitting global parameters found in the crime data set ($s = 2.8 \times 10^6$, $\alpha = 0.93$) when fitting to the patent dataset. The comparison of our theory with the empirical patent data is shown in Fig. S8. Our model predicts similar superlinear scaling behavior shown in the data, suggesting that our model can be generalized to urban outputs beyond crime.

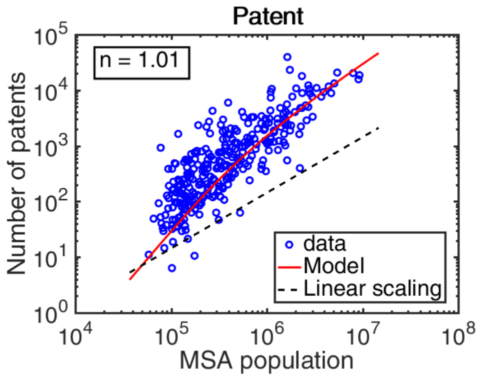


**Figure S8:** The fit of the model to patent scaling data in year 2000, using the best fitting $\alpha$ and $s$ parameters found by fitting to crime scaling and co-offending group sizes in the NIBRS dataset.

# 10 Code and data availability

Code used in parameter fitting and generating the scaling laws fit figures, as well as the data input needed, can be accessed from the repository: `https://github.com/vc-yang/urban_productivity_scaling_laws`.

# References

[1] US Department of Justice. Federal Bureau of Investigation, "Uniform crime reporting program data: National incident-based reporting system," 2014. Data retrieved from Ann Arbor, MI: Inter-university Consortium for Political and Social Research in March 2017. http://doi.org/10.3886/ICPSR36398.v1.

[2] W. W. Cohen, "Enron email dataset," 2014. Data retrieved from `http://www.cs.cmu.edu/~enron/`.

[3] US Federal Bureau of Investigation, "Crime in the United States, 1999 – 2013," 1999 – 2013.

[4] L. M. A. Bettencourt, J. Lobo, D. Helbing, C. Kühnert, and G. B. West, "Growth, innovation, scaling, and the pace of life in cities," *Proceedings of the National Academy of Sciences*, vol. 104, no. 17, pp. 7301–7306, 2007.

[5] R. I. Dunbar, "Cognitive constraints on the structure and dynamics of social networks.," *Group Dynamics: Theory, Research, and Practice*, vol. 12, no. 1, p. 7, 2008.

[6] J. C. Leitao, J. M. Miotto, M. Gerlach, and E. G. Altmann, "Is this scaling nonlinear?," *Royal Society Open Science*, vol. 3, no. 7, p. 150649, 2016.

[7] A. Gomez-Lievano, O. Patterson-Lomba, and R. Hausmann, "Explaining the prevalence, scaling and variance of urban phenomena," *Nature Human Behavior*, vol. 390, no. 11, pp. 2155–2159, 2017.

[8] E.-J. Wagenmakers and S. Farrell, "AIC model selection using Akaike weights," *Psychonomic Bulletin & Review*, vol. 11, no. 1, pp. 192–196, 2004.

[9] E. D. Gould, B. A. Weinberg, and D. B. Mustard, "Crime rates and local labor market opportunities in the united states: 1979–1997," *Review of Economics and Statistics*, vol. 84, pp. 45–61, 2002.

[10] J. Grogger, "Market wages and youth crime, no. w5983," *National Bureau of Economic Research*, 1997.

[11] S. Machin and C. Meghir, "Crime and economic incentives," *Journal of Human Resources*, vol. 39, no. 4, pp. 958–979, 2004.

[12] L. M. A. Bettencourt, "The origins of scaling in cities," *Science*, vol. 340, no. 6139, pp. 1438–1441, 2013.

[13] B. H. Hall, A. B. Jaffe, and M. Trajtenberg, "The NBER patent citation data file: Lessons, insights and methodological tools," tech. rep., National Bureau of Economic Research, 2001.

[14] L. M. A. Bettencourt, J. Lobo, and D. Strumsky, "Invention in the city: Increasing returns to scale in metropolitan patenting," *Los Alamos National Laboratory technical Report LAUR-04-8798*, 2004.
